# Supplementary material for: MalAlgoQA: Pedagogical Evaluation of Counterfactual Reasoning in Large Language Models and Implications for AI in Education
Source: arXiv:2407.00938 source file (2024-10-05)
Supplement: Supplementary file 1 [file appendix_examples.tex]

\begin{table*}[ht!]
\centering
\begin{minipage}[t]{1\textwidth}
\begin{lstlisting}[mathescape=true,basicstyle=\ttfamily\smalltonormalsize]
$\textbf{Reading Question Set Example 1}$: 

Content Classification: Literature

Passage: Blueberries
          1 You ought to have seen what I saw on my way 
          2 To the village, through Patterson's pasture to-day: 
          3 Blueberries as big as the end of your thumb, 
          4 Real sky-blue, and heavy, and ready to drum 
          5 In the cavernous pail of the first one to come! 
          6 And all ripe together, not some of them green 
          7 And some of them ripe! You ought to have seen!
            ...
            
Question: In lines 1-7, the speaker expresses great surprise about the ...?

Answer and Rationales:
$\colorbox{lightyellow}{A: large pails of blueberries.}$
Rationale A: Some readers might find this option plausible because the speaker mentions the ``cavernous pail of the first one to come" (line 5). However, this mention of the pail is referring to the pail into which the lucky picker who first stumbles across this crop will put the ``Blueberries as big as the end of your thumb" (line 3). The speaker does not express surprise that pickers are bringing large pails.
$\colorbox{lightyellow}{B: number of blueberry pickers.}$
Rationale B: Some readers might choose this option because the phrase ``the first one to come" in line 5 refers to a blueberry picker. However, although the speaker is predicting success for anyone who comes to pick the blueberries, the speaker is not expressing surprise that there are no pickers yet. Based on the speaker's description of how big, blue, and ripe the berries are (``as big as the end of your thumb, Real sky-blue, and heavy, and ready" (lines 3 and 4)), the berries are undisturbed, and no one has discovered them except for the speaker.
$\colorbox{lightyellow}{C: ripeness of the blueberries.}$
Rationale C: The speaker describes ``big as the end of your thumb" (line 3) blueberries that are ``Real sky-blue, and heavy," (line 4) and ``all ripe together" (line 6). The speaker repeats, ``You ought to have seen" in lines 1 and 7 to convey surprise.
$\colorbox{lightyellow}{D: size of new blueberry bushes.}$
Rationale D: This option might seem plausible because the size of the blueberries and their bushes are described. The first speaker draws attention to size when describing the blueberries as ``big as the end of your thumb" (line 3). In line 13, the second speaker exclaims, ``Why, there hasn't been time for the bushes to grow." This line implies that the bushes must be small, so it is surprising that the blueberries they produce are numerous and ``as big as the end of your thumb." Although lines 1-7 address the blueberries, the speaker does not mention the bushes on which they grow in those lines.

\end{lstlisting}
\end{minipage}
\hfill
\caption{Example 1 of Reading question set. }
\label{tab:reading_example-1}
\end{table*}

\begin{table*}[ht!]
\centering
\begin{minipage}[t]{1\textwidth}
\begin{lstlisting}[mathescape=true,basicstyle=\ttfamily\smalltonormalsize]
$\textbf{Reading Question Set Example 2}$: 

Content Classification: Informational Text

Passage: Creating Codes: Grace Hopper and the Computer Compiler 
          1 The computer screen freezes. No matter what or how often you click, the hourglass or rotating circle (that symbol that insists, ``I'm working on it!") spins away. You want to shake the screen. Someone next to you says, ``I think you found a bug." 
          ...
            
Question: What is the main purpose of paragraph 1?

Answer and Rationales:
$\colorbox{lightyellow}{A: To demonstrate the importance of the subject}$
Rationale A: Although some readers may conclude that the frozen computer screen in paragraph 1 demonstrates how important computer programming is currently, the paragraph describes a familiar feeling of frustration rather than detailing the more serious consequences that could result from programming mistakes.
$\colorbox{lightyellow}{B: To help readers make a connection with the topic}$
Rationale B: The paragraph describes a person facing a frozen computer screen that many readers have probably experienced in order to help readers make a personal connection to the topic. By describing this common situation, the reader's interest is engaged. So, when the article continues on to discuss Hopper's contribution to programming and how she helped solve some of the early computer bugs, readers feel more connected with the topic.
$\colorbox{lightyellow}{C: To give background information about the subject}$
Rationale C: Although introductions often provide background information, and some readers may conclude that explaining a computer bug is background information for the article, the topic of the article focuses not on computer bugs but on Hopper's contributions to computer programming.
$\colorbox{lightyellow}{D: To provide readers with a brief summary of the topic}$
Rationale D: Although the main topic of the article is Hopper's contribution to computer programming and paragraph 1 mentions computers, paragraph 1 describes a common situation in order to raise interest among readers. It describes a person having computer problems rather than summarizing Hopper's contributions to computer programming.

\end{lstlisting}
\end{minipage}
\hfill
\caption{Example 2 of Reading question set}
\label{tab:reading_example-2}
\end{table*}
